# Supplementary material for: OctGPT: Octree-based Multiscale Autoregressive Models for 3D Shape Generation
Source: arXiv:2504.09975 source file (2025-04-15)
Supplement: Supplementary file 1 [file logs.tex]

\section{Working Logs} \label{app:sec:logs}

\subsection{Week 1 Project Meeting - 20240909} \label{app:sec:w1}

We discussed the project idea and motivation.
ST wrote the first version of the introduction.

\subsection{Week 2 Project Meeting - 20240916} \label{app:sec:w2}

\paragraph{PS}
Our initial goal is to train masked autoregressive model on octrees.
For masked autoregressive models, we should carefully read and understand the following papers: MaskGIT~\cite{Chang2022}, D3PM, and MaskAR (in Kaiming's paper).

\paragraph{Wei Sitong}: I have finished the first draft of the introduction. I tried a simple model which predicts split signals in depth4, but the model can only generate one average octree. I will try the mask-generate paradigm in the next week.

\subsection{Week 3 Project Meeting - 20240923} \label{app:sec:w3}

\paragraph{PS}
We can first train a model to predict the split signals ($0/1$) in the octree on voxels with a resolution of $16^3$ or $8^3$.
In \cref{fig:var}, we can see the visualization of the VAR model. The key difference VAR and our method is that VAR predicts all the split signals in the next scale, we instead predict the next-k signals following MaskAR.

\begin{figure}
    \centering
    \includegraphics[width=0.8\columnwidth]{var.png}
    \caption{Visualization of the VAR model.}
    \Description{VAR model.}
    \label{fig:var}
\end{figure}

\paragraph{Wei Sitong}: This week I have tried the mask-generate paradigm. The 8-channel split signals are represented as a 256-category classification. I found the results are not satisfying. The reconstruction results with $\le 0.9$ mask ratio are as-expected. However, the generation results with $1.0$ mask ratio are all average meshes.

\subsection{Week 3 Group Meeting - 20240927}

\paragraph{PS}
Considering that MaskGIT has not yielded satisfactory results and we will eventually not choose MaskGIT, I suggest we promptly return to the solution we discussed. There is no need to spend more time on adjusting MaskGIT.

The autoregressive models (AR) have standardized implementations. We can first train a model with AR on the full voxel grid. Then, we can \emph{modify the causal mask} in the AR to implement our method.

Alternatively, we can also run the masked autoregressive Models (MAR). Our differences from MAR are: (1) We do not predict tokens in a random order; (2) We predict tokens of multiple resolutions.
When transitioning from one resolution to the next, we follow the rule of octree splitting to subdivide each node into 8.

The third option is to run the code of VAR.
We could first run experiments on the full voxel grid with VAR, and then modify VAR’s causal mask to implement our method.
We do not need VAR's subdivision method; we have our own octree splitting method for subdivision.

\paragraph{Wei Sitong}: The paradigm following MaskGIT seems not work. The following methods are considered: next-k prediction (like GPT), next-scale prediction (like VAR), and next-k prediction with mask-generate (like MAR). I think Chenyu, Yiming, Mingyang and I can each complete one method and compare the results.

Next-k prediction: The codebase is LlamaGen (Autoregressive beats diffusion). The model will predict the next-k split signals in z-order. We can firstly conduct the experiments on 16x16x16 voxels with normal transformers, then we can try the octree transformers.

Next-scale prediction: The codebase is VAR. The full depth will be set to zero and the octree will be predicted from the root. The split loss will be calculated on each scale. That's because to generate octree with diversity, sampling in only one scale is not enough.

Next-k prediction with mask-generate: The codebase is MAR. The model will predict the next-k split signals in random-order. The mask-generate paradigm will be used to generate the octree.

According to my observation in experiments, I think the split signals are not similar with VQVAE tokens. Different VQVAE tokens might have overlapping area in distribution, but split signals are totally discrete. That means noise in VQVAE tokens might be corrected by the decoder, while noise in split signals will be remained and propagated to the next scale.

\subsection{Week 4 Project Meeting - 20241007} \label{app:sec:w4}
\paragraph{Wei Sitong}: I continued the experiments on MAR. I choose MAR as the basic framework because its code has been well-organized. I believe GPT paradigm is similar to MAR paradigm, if we can not achieve good results on MAR, we can not achieve good results on GPT neither.

I firstly conducted the experiments generating depth5 from depth4. The results are satisfying in both quality and diversity. Then I conducted the depth4-depth6 generation, some generated meshes have good quality and diversity but some have more noise. I also found that diversity can be improved by random generated order.

\subsection{Week 5 Project Meeting - 20241015} \label{app:sec:w5}
\paragraph{Wei Sitong}: I implemented the simple GPT paradigm based on the 3DILG, and perform experiments on depth4-depth5 generation. The quality of generated octree is satisfying, and the diversity is very good (I think it is better than diffusion). Then I concatenated the depth4 and depth5 split and performed the depth4-depth6 generation. The sequence length are not fixed, so I have to use bs=1 now. The inference time for GPT is very long, and the memory consumption is very large. I'm trying to learn some advanced techniques(KV-cache and flash attention) to improve the performance.

\subsection{Week 6 Project Meeting - 20241022} \label{app:sec:w6}
\paragraph{Wei Sitong}: This week I tried to implement the octree window attention to accelerate GPT. At first, I set the window size to 26, but the results are not satisfying. Then I set a larger window size(1024/2048), the results are better, but still not as good as causal attention. I also found that the loss of window attention is slightly larger than causal attention. I think these results might be too noisy to generate high quality meshes by VQVAE, so I have to find some ways to reduce the noise.

\subsection{Week 7 Project Meeting - 20241029} \label{app:sec:w7}
\paragraph{Wei Sitong}: This week I connected the VQVAE and GPT to generate meshes. I moved the core code to `thsolver' framework, because the original framework (from SDFusion) is too complex. I found that the VQVAE checkpoint was trained on depth3-8 octree, so I train a new GPT generating depth3-6 splits and got better results than previous depth4-6 experiments. Then I tried the depth3-6+VQVAE experiments, and the generated meshes are satisfying. However, the generation process is `very very very' slow. So I think KV-cache must be implemented next.
